# Supplementary material for: Swift4D:Adaptive divide-and-conquer Gaussian Splatting for compact and efficient reconstruction of dynamic scene
Source: arXiv:2503.12307 source file (2025-03-16)
Supplement: Supplementary file 1 [file 8_appendix.tex]

In the supplementary materials, we will provide more details. In Sec.\ref{sec:implement details}, we provide  detailed setting s about our method. In Sec.\ref{appendix sec: dynamic - static  separation}, we describe our dynamic-static decomposition method in detail. In Sec.\ref{appendix sec: more result}, we present additional experimental results.

\subsection{ Implement details}
\label{sec:implement details}
\textbf{Three-stage method.} In the first stage, we train the Gaussian points initialized by SfM\cite{schonberger2016structure} using the first frame images from each viewpoint. The goal of this stage is to obtain a canonical space. In the second stage, we train the dynamic parameter \(d\) of each Gaussian point according to the method proposed in Sec. \ref{sec:segmentation}. In the third stage, we jointly train the attributes of the Gaussian points and the spatio-temporal structure.

\textbf{MLPs as feature decoders.} As shown in Fig.\ref{figs:muti head mlp}. we use five shallow MLPs as decoders for the mean, opacity, color, rotation, and scaling, respectively. The outputs are directly added to the attributes of the Gaussian points in the canonical space, and then passed through the corresponding activation functions to obtain the attributes at time t.

\textbf{Lite version.} We empirically found that removing the SSIM loss, while slightly degrading rendering quality, offers the advantage of reducing the number of Gaussian points by 2-3 times (approximately 200,000). Therefore, we removed the SSIM loss and set the hash table size to \(2^{15}\) in the Lite version. This ensures a significant reduction in model size without severely impacting rendering quality. The models rendered in the Lite version average only 30MB in size, with the Gaussian point cloud being 22MB and the hash table 8MB, making it the smallest dynamic model to date (including the NeRF series).

\subsection{ dynamic - static  decomposition}
\label{appendix sec: dynamic - static  separation}
We precompute the temporal variance \( S^2_i(x) \) for each pixel \( x \in \mathbf{R} \) to generate the variance map \( V_i \) for each viewpoint \( i \). To reduce noise, we smooth \( V_i \) using a Gaussian filter with a 31x31 kernel. Each pixel's variance \( S^2_i(x) \) is then binarized into \( D_i(x) \) using a threshold \( \gamma \), providing pixel-level supervision.

Initially, the dynamic parameter \( d \) of each Gaussian point is set to 0, resulting in a dynamic value of \(\hat D_i(x) = 0.5\) for each pixel. 
When the cross-entropy loss \(\mathcal{L}_d\) is employed as the loss function, the Gaussian points that intersect with the dynamic pixel \( \hat{D}_i(x) \) will receive a positive gradient, leading to the dynamic parameter \(d\) expanding towards \( +\infty \).  Conversely, when Gaussian points intersect with static pixels, the dynamic parameter \( d \) will expand towards \( -\infty \). Due to the properties of the \textbf{Sigmoid} function, the dynamic parameter can extend infinitely towards both \( -\infty \) and \( +\infty \), allowing us to better distinguish between dynamic and static points. 

When a Gaussian point intersects both dynamic and static pixels (e.g., in the presence of occlusion), it will receive two opposing gradient values. If the positive gradient is larger, its dynamic value will be greater than 0, classifying it as a dynamic point. Conversely, if the negative gradient dominates, it will be classified as a static point. 

Finally, we provide the formula for calculating the gradient received by each Gaussian point. Based on this formula, the CUDA code can be easily written. Assuming we need to compute the dynamic value gradient of Gaussian point \(g\), the equation as following: \(\frac{\partial \mathcal{L}_d}{\partial d_g}\). Due to \textit{autograd} , we have known \(grad_1\):
\begin{equation}
    grad_1 = \frac{\partial \mathcal{L}_d}{\partial (\sum_{i=1}d_i \alpha_i' \prod_{j=1}^{i-1}(1-\alpha_j')) }
\end{equation}
 we only need to compute:
\begin{equation}
    grad_2 = \frac{\partial (\sum_{i=1}d_i \alpha_i' \prod_{j=1}^{i-1}(1-\alpha_j'))}{\partial d_g} = ( \alpha_g' \prod_{j=1}^{g-1}(1-\alpha_j') )
\end{equation}
So, the final formula is as follows:
\begin{align}
    \frac{\partial \mathcal{L}_d}{\partial d_g} &= \frac{\partial \mathcal{L}_d}{\partial (\sum_{i=1}d_i \alpha_i' \prod_{j=1}^{i-1}(1-\alpha_j')) } *\frac{\partial (\sum_{i=1}d_i \alpha_i' \prod_{j=1}^{i-1}(1-\alpha_j'))}{\partial d_g}  \\
 &= \frac{\partial \mathcal{L}_d}{\partial (\sum_{i=1}d_i \alpha_i' \prod_{j=1}^{i-1}(1-\alpha_j')) } * ( \alpha_g' \prod_{j=1}^{g-1}(1-\alpha_j')   )
\end{align} 

From this formula, it can be seen that the gradient of the dynamic value is related to occlusion, self-opacity, and the distance to the camera plane, which is very reasonable.

\subsection{ More results }
\label{appendix sec: more result}

Fig.\ref{fig: different itreation compaire} shows the rendering results from new viewpoints at different iteration of training. It can be observed that our method achieves very high quality after 7000 epochs (approximately 10 minutes), demonstrating that our approach is highly efficient for reconstructing 4D dynamic scenes. Fig.\ref{fig: dynamic mask compaire} demonstrates that our method can effectively segment dynamic points. Tab. \ref{tab: basketball} presents the results of several static and dynamic methods on the basketball court dataset\cite{VRU}, showing that our method outperforms 4DGS\cite{wu20244d}. To demonstrate the robustness and generalization of our approach, we also conducted experiments on the ENeRF dataset. The results, shown in Table~\ref{tab:enerf dataset}, follow the training policies described in 4k4d \cite{xu20244k4d}.

% 1. 周期性渲染图  证明收敛快  3000 7000  13000 GT

\begin{figure}[t]
\centering
\setcounter{subfigure}{0}  % 序号清零
\subfloat{\includegraphics[scale=0.071]{figs/appendix/all_scene/coffee/00150.png}}
\hfill
\subfloat{\includegraphics[scale=0.071]{figs/appendix/all_scene/coffee/3000_150.png}}
\hfill
\subfloat{\includegraphics[scale=0.071]{figs/appendix/all_scene/coffee/7000_150.png}}
\hfill
\subfloat{\includegraphics[scale=0.071]{figs/appendix/all_scene/coffee/13000_150.png}}

\subfloat{\includegraphics[scale=0.071]{figs/appendix/all_scene/cut_beef/00150.png}}
\hfill
\subfloat{\includegraphics[scale=0.071]{figs/appendix/all_scene/cut_beef/3000_150.png}}
\hfill
\subfloat{\includegraphics[scale=0.071]{figs/appendix/all_scene/cut_beef/7000_150.png}}
\hfill
\subfloat{\includegraphics[scale=0.071]{figs/appendix/all_scene/cut_beef/13000_150.png}}

\subfloat{\includegraphics[scale=0.071]{figs/appendix/all_scene/flame_salmon/00250.png}}
\hfill
\subfloat{\includegraphics[scale=0.071]{figs/appendix/all_scene/flame_salmon/3000_250.png}}
\hfill
\subfloat{\includegraphics[scale=0.071]{figs/appendix/all_scene/flame_salmon/7000_250.png}}
\hfill
\subfloat{\includegraphics[scale=0.071]{figs/appendix/all_scene/flame_salmon/13000_250.png}}

\subfloat{\includegraphics[scale=0.071]{figs/appendix/all_scene/flame_steak/00189.png}}
\hfill
\subfloat{\includegraphics[scale=0.071]{figs/appendix/all_scene/flame_steak/3000_189.png}}
\hfill
\subfloat{\includegraphics[scale=0.071]{figs/appendix/all_scene/flame_steak/7000_189.png}}
\hfill
\subfloat{\includegraphics[scale=0.071]{figs/appendix/all_scene/flame_steak/13000_189.png}}

\subfloat{\includegraphics[scale=0.071]{figs/appendix/all_scene/sear_steak/00150.png}}
\hfill
\subfloat{\includegraphics[scale=0.071]{figs/appendix/all_scene/sear_steak/3000_150.png}}
\hfill
\subfloat{\includegraphics[scale=0.071]{figs/appendix/all_scene/sear_steak/7000_150.png}}
\hfill
\subfloat{\includegraphics[scale=0.071]{figs/appendix/all_scene/sear_steak/13000_150.png}}

\setcounter{subfigure}{0}  % 序号清零
\subfloat[GT]{\includegraphics[scale=0.071]{figs/appendix/all_scene/spinach/00121.png}}
\hfill
\subfloat[3000 its]{\includegraphics[scale=0.071]{figs/appendix/all_scene/spinach/3000_121.png}}
\hfill
\subfloat[7000 its]{\includegraphics[scale=0.071]{figs/appendix/all_scene/spinach/7000_121.png}}
\hfill
\subfloat[13000 its]{\includegraphics[scale=0.071]{figs/appendix/all_scene/spinach/13000_121.png}}

\caption{\textbf{Training Epoch Comparison:} the results of our method in 3000, 7000, 13000 epochs. Based on the results from 3000 iterations, our method demonstrates rapid convergence. }
\label{fig: different itreation compaire}
\end{figure}

\begin{figure}[t]
    \centering
    \includegraphics[width= \textwidth ,trim=1cm 1cm 17.5cm 0.5cm]{figs/appendix/dynamic_mask/all_dynamic_mask.pdf}
    
\caption{\textbf{Decomposition results}. (a) is the dynamic-static pixel mask, (b) is the dynamic map rendered with our dynamic value \(d\) of Gaussians, (c) is the image rendered with dynamic Gaussians, and (d) is the GT image.}
\label{fig: dynamic mask compaire}
\end{figure}

\begin{figure}[t]
    \centering
    \includegraphics[width= \textwidth ,trim=1cm 2cm 10cm 5cm]{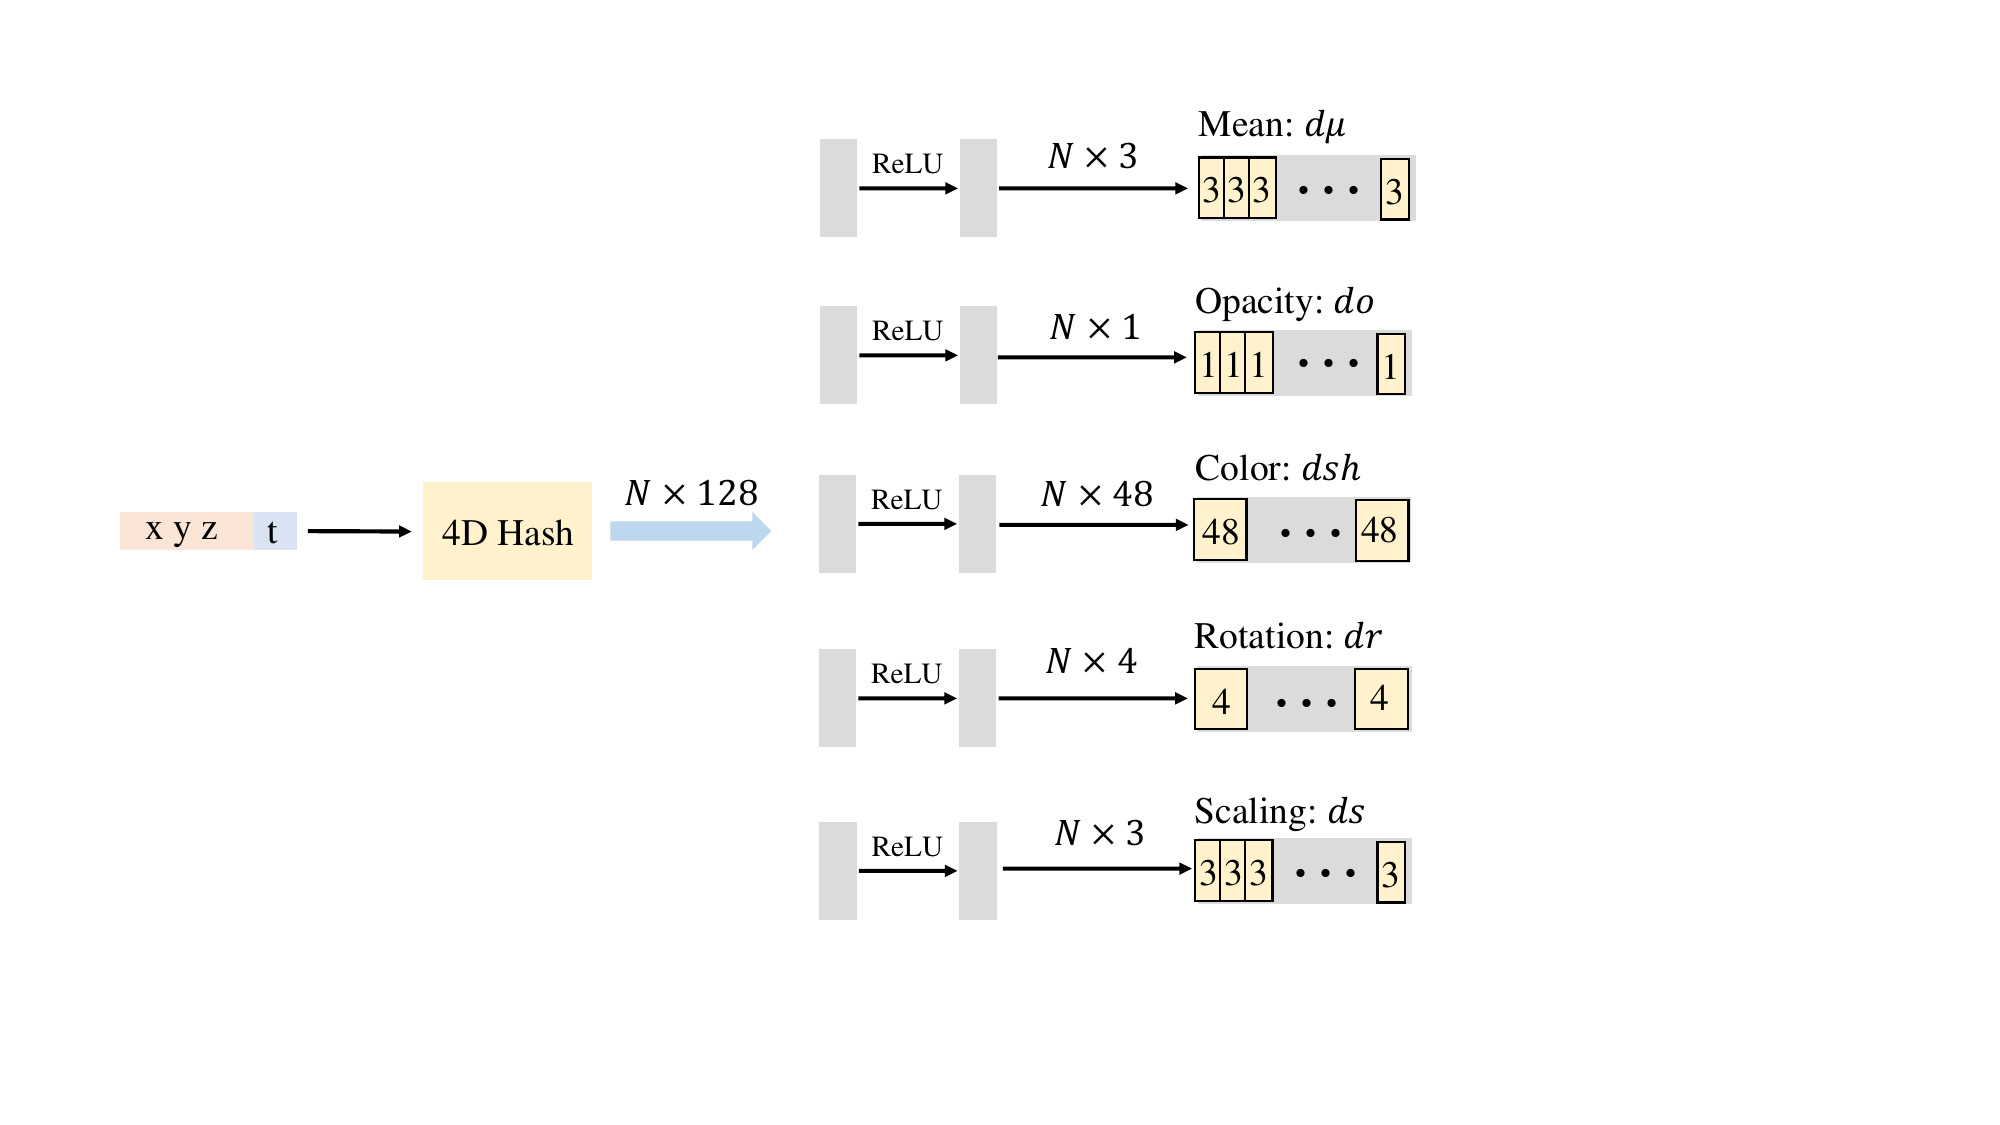}
    \caption{\textbf{MLP Structures.} For each dynamic point, we use five small MLPs to predict the deformations.}
    \label{figs:muti head mlp}
\end{figure}

\begin{table}[t]
    \centering
	% \aboverulesep=0pt
	% \belowrulesep=0pt
    \caption{\textbf{ Per-scenes results on the NV3D dataset.} The best and the second best results are denoted by \textcolor{red!50}{red} and \textcolor{blue!50}{blue}.}
    \label{tab: per scene result on nv3d}
    \begin{threeparttable}
    \resizebox{\textwidth}{!}
    {
        \begin{tabular}{ccccccccccccc}
        \toprule[1.5pt]
         Method &Coffee Martini & Spinach & Cut Beef & Flame Salmon & Flame Steak & Sear Steak & Mean\\

        \midrule[0.5pt]
        \multirow{1}{*}{MixVoxels } & \cellcolor{blue!25}29.36 &31.61& 31.30 &\cellcolor{red!25}29.92 &31.21 &31.43 &30.80\\
        
        \multirow{1}{*}{NeRFPlayer }&  31.53& 30.56 & 29.35&  31.65 & 31.93 & 29.13 &  30.69\\

        \multirow{1}{*}{HexPlane } &  --&  32.04&  32.55 & 29.47 & 32.08 & 32.39&  31.70\\

        \multirow{1}{*}{K-Planes } & \cellcolor{red!25}{29.99} & 32.60&  31.82 & 30.44 & 32.38&  32.52&  31.63\\

        \multirow{1}{*}{4DGS}  & 27.34  &32.46  &32.90& 29.20 & 32.51 & 32.49 & 31.15 \\

        \multirow{1}{*}{3DGStream } & 27.75 &\cellcolor{red!25}{33.31} &33.21&28.42& \cellcolor{red!25}{34.30} & 33.01  & 31.67 \\

        \multirow{1}{*}{SpaceTimeGS}  & 28.61 & 33.18 & 33.52 & 29.48 & 33.64  &\cellcolor{blue!25}33.89 & \cellcolor{blue!25}32.05\\
        
        \multirow{1}{*}{Real-Time4DGS }  & 28.33& 32.93& \cellcolor{red!25}{33.85} & 29.38 &\cellcolor{blue!25}34.03 &33.51& 32.01 \\
        \multirow{1}{*}{\textbf{\confDataName Lite(Ours)}}  &  28.84	& 	32.57& 	32.82& 	\cellcolor{red!25}{29.92} & 33.13	& 33.48& 	31.79\\
        
        \multirow{1}{*}{\textbf{\confDataName(Ours)}}  & 29.13	&\cellcolor{blue!25}33.05&	\cellcolor{blue!25}33.80 &	\cellcolor{blue!25}29.75 &	33.67	&\cellcolor{red!25}{33.98}	& \cellcolor{red!25}{32.23}  \\

        \bottomrule[1.5pt]
        \end{tabular}
    }
    
\end{threeparttable}
\end{table}

\begin{table}[t]
    \centering
    \caption{\textbf{Quantitative comparison on the Basketball court dataset.} The first four methods correspond to static methods, tested on the first frame, while the last two methods represent dynamic methods, tested on 20 frames.}
    \label{tab: basketball}
    \begin{threeparttable}
    \resizebox{0.7\textwidth}{!}
    {
        \begin{tabular}{ccccccccccccc}
        \toprule[1.5pt]
         Method & PSNR \(\uparrow\)  & SSIM \(\uparrow\) \(\downarrow\)  & LPIPS \(\downarrow\) \\
        \midrule[0.5pt]
        \multirow{1}{*}{Gof \cite{yu2024gaussian} }  & 30.39 & 0.949 & 0.141 \\
        \multirow{1}{*}{2DGS \cite{huang20242d} }  & 30.78 & 0.949 & 0.187 \\
        \multirow{1}{*}{PixelGS  \cite{zhang2024pixel}}  & 29.26 & 0.946 & 0.168 \\
        \multirow{1}{*}{3DGS\cite{kerbl20233d}}  & 30.50 & 0.949 & 0.171 \\
        \midrule[0.5pt]
        \multirow{1}{*}{4DGS\cite{wu20244d} }  & 27.87 & 0.921 & 0.191 \\
        \multirow{1}{*}{\textbf{\confDataName(Ours)}}  & 29.03 & 0.933 & 0.187  \\
        \bottomrule[1.5pt]
        \end{tabular}
}
\end{threeparttable}
\end{table}

% \begin{figure}[t]
% \centering
% \setcounter{subfigure}{0}  % 序号清零
% \subfloat{\includegraphics[scale=0.071]{figs/appendix/decomposition/00000.png}}
% \hfill
% \subfloat{\includegraphics[scale=0.071]{figs/appendix/decomposition/00050.png}}
% \hfill
% \subfloat{\includegraphics[scale=0.071]{figs/appendix/decomposition/00100.png}}
% \hfill
% \subfloat{\includegraphics[scale=0.071]{figs/appendix/decomposition/00120.png}}

% \setcounter{subfigure}{0}  % 序号清零
% \subfloat{\includegraphics[scale=0.071]{figs/appendix/decomposition/00150.png}}
% \hfill
% \subfloat{\includegraphics[scale=0.071]{figs/appendix/decomposition/00180.png}}
% \hfill
% \subfloat{\includegraphics[scale=0.071]{figs/appendix/decomposition/00200.png}}
% \hfill
% \subfloat{\includegraphics[scale=0.071]{figs/appendix/decomposition/00299.png}}

% \caption{The result of hierarchical rendering in dynamic scenes based on the dynamic parameter \(d\) of Gaussian points. The specific video can be found in the supplementary material.}
% \label{fig: appendix decomposition}
% \end{figure}

\begin{table}[t]
\centering
\caption{ \textcolor{orange}{Performance comparison of different methods on ENeRF dataset. The results are derived from 4k4d.}
}
\begin{tabular}{lccc}
\hline
\textbf{Methods} & \textbf{PSNR} $\uparrow$ & \textbf{SSIM} $\uparrow$ & \textbf{LPIPS} $\downarrow$ \\
\hline
ENeRF \cite{lin2022efficient} & 25.452 & 0.809 & 0.273 \\
IBRNet \cite{wang2021ibrnet} & 24.966 & \cellcolor{orange!100}0.929 & 0.172 \\
KPlanes \cite{fridovich2023k} & 21.310 & 0.735 & 0.454 \\
4k4d \cite{xu20244k4d} & 25.815 & 0.898 & 0.147 \\
Swift4D (Ours) & \cellcolor{orange!100}26.12 & 0.911 & \cellcolor{orange!100}0.070 \\
\hline
\end{tabular}
\label{tab:enerf dataset}
\end{table}

\begin{figure}[t]
    \centering
    \includegraphics[width= \textwidth ,trim=0cm 8cm 7cm 0cm]{figs/appendix/decomposition/decomposition.pdf}
\caption{The result of hierarchical rendering in dynamic scenes based on the dynamic parameter \(d\) of Gaussian points. The specific video can be found in the supplementary material.}
\label{fig: appendix decomposition}
\end{figure}

% \begin{figure}[t]
% \centering

% \subfloat{\includegraphics[scale=0.046]{figs/compare/basketball/00007_gt.png}}
% \hfill
% \subfloat{\includegraphics[scale=0.046]{figs/compare/basketball/00022_gt.png}}
% \hfill
% \subfloat{\includegraphics[scale=0.046]{figs/compare/basketball/00037_gt.png}}
% \hfill
% \subfloat{\includegraphics[scale=0.046]{figs/compare/basketball/00052_gt.png}}

% \setcounter{subfigure}{0}  % 序号清零
% \subfloat[view 1]{\includegraphics[scale=0.046]{figs/compare/basketball/00007.png}}
% \hfill
% \subfloat[view 2]{\includegraphics[scale=0.046]{figs/compare/basketball/00022.png}}
% \hfill
% \subfloat[view 3]{\includegraphics[scale=0.046]{figs/compare/basketball/00037.png}}
% \hfill
% \subfloat[view 4]{\includegraphics[scale=0.046]{figs/compare/basketball/00052.png}}

% \caption{The training results of the basketball court from four novel viewpoints. The images above are the GT images, and the ones below are our rendered results. }
% \label{fig: appendix basketball}
% \vspace{-1em}
% \end{figure}

\begin{figure}[t]
    \centering
    \includegraphics[width= \textwidth ,trim=0cm 9cm 1cm 0cm]{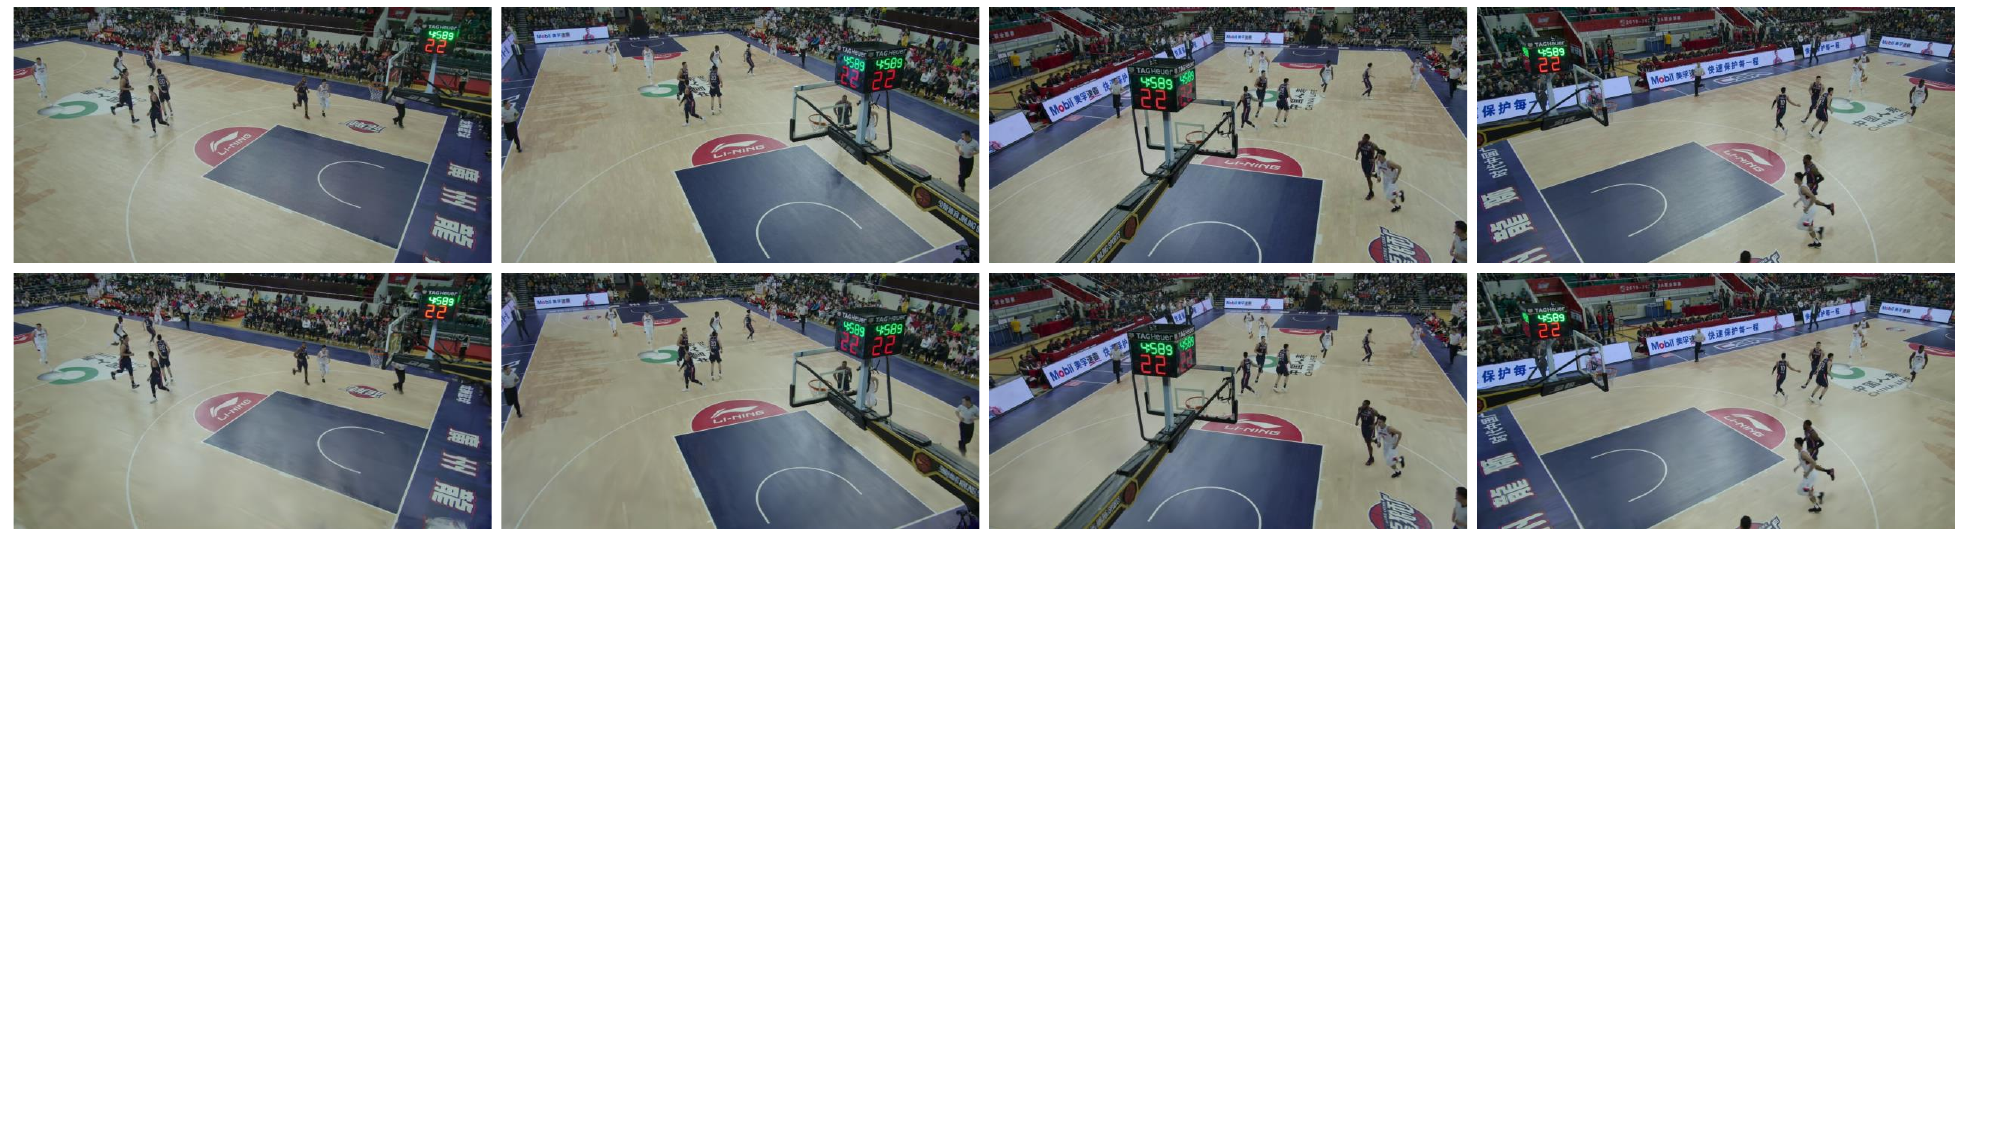}
\caption{The training results of the basketball court from four novel viewpoints. The images above are the GT images, and the ones below are our rendered results. }
\label{fig: appendix basketball}
\end{figure}
